# Supplementary material for: Tight bounds on the mutual coherence of sensing matrices for Wigner D-functions on regular grids
Source: arXiv:2010.02344 source file (2020-10-05)
Supplement: Supplementary file 1 [file supplementary.tex]

\subsection{Spherical Harmonics and Wigner-D Functions}
In this section, the spherical harmonics as the homogeneous solution of Laplace equation is derived where the content is mainly taken from Lebedev \cite{silverman1972special} and classical book of Courant and Hilbert in the mathematical physics \cite{hilbert2004methods}. In addition, the material related to the Laplace equation in the rotation group is given by \cite{kyatkin2000engineering}. Before starting to find homogeneous solution of Laplace equation in the unit sphere $\mathrm{S}^2$, for simplicity, the homogeneous solution of Laplace equation in the unit circle $\mathrm{S}^1$ will be reviewed instead. It is well known that Fourier series is the solution of Laplacian on $\mathbb{R}^2$ which could be expressed in cartesian cooridnate as the following
\begin{equation}
\Delta f = \frac{\partial^2 f}{\partial x^2} + \frac{\partial^2 f}{\partial y^2}
\end{equation}
where $f: \mathbb{R}^2 \rightarrow \mathbb{R}$. In polar coordinate, by using the relation $(x,y) = (r\cos \theta, r\sin \theta)$ with $r > 0$, the Laplacian is given by 
\begin{equation}
\Delta f = \frac{1}{r}\frac{\partial}{\partial r}\bigg(r \frac{\partial f}{\partial r} \bigg) + \frac{1}{r^2}\frac{\partial^2 f}{\partial \theta^2} 
\end{equation}
On the unit circle $\mathrm S^1 = \{(x,y) \in \mathbb{R}^2 |\,\,  x^2 + y^2 = 1\}$, we have the Laplacian 
\begin{equation}
\Delta_{\mathrm S^1} f =   \frac{\partial^2 f}{\partial \theta^2} 
\end{equation}
For the sake simplicity, let us consider a homogeneous function of degree $l$, which is $f(r,\theta) = r^l g(\theta)$. Applying this function into Laplacian in polar coordinate, we will get
\begin{equation}
    \Delta_f = r^{l-2}(l^2 g + \Delta_{\mathrm S^1 g})
\end{equation}
It can be seen that, the solution of Laplace equation is achieved as the following
\begin{equation}
    \Delta_{\mathrm S^1} g = -l^2g
\end{equation}
where $g$ is an eigenfunction of $\Delta_{\mathrm S^1}$ for eigenvalue $-l^2$  where the general solution is given by
\begin{equation}
    g(\theta) = a_n \cos l \theta + b_n \sin l \theta 
\end{equation}
for $l \geq 0$. This general solution is the Fourier series with $a_n , b_n$ as the Fourier coefficients. Now if we extend the problem into higher dimension on unit sphere $\mathrm{S}^2 = \{(x,y,z) \in \mathbb{R}^2 |\,\, x^2 +y^2 +z^2 = 1\}$, the general solution of Laplace equation is the spherical harmonics. First of all, the Laplacion in $\mathbb{R}^3$ is given by
\begin{equation}
    \Delta_f = \frac{\partial^2 f}{\partial x^2} + \frac{\partial^2 f}{\partial y^2} +\frac{\partial^2 f}{\partial z^2}
\end{equation}
By using cartesian  to spherical coordinates transformation 
\begin{equation*}
    x = r \sin \theta \cos \phi \,\,,
    y = r \sin \theta \sin \phi \,\,,
    z = r \cos \theta
\end{equation*}
where $\theta \in [0,\pi]$ and $\phi \in [0,2\pi)$ and $r > 0$, the Laplacian in spherical coordinates is given by
\begin{equation}
\Delta f = \frac{1}{r^2}\frac{\partial}{\partial r}\bigg(r^2 \frac{\partial f}{\partial r} \bigg) + \frac{1}{r^2}\Delta_{\mathrm{S}^2 f}
\end{equation}
where, 
\begin{equation}
\Delta_{\mathrm{S}^2} f =  \frac{1}{\sin \theta} \frac{\partial}{\partial \theta} \bigg( \sin \theta \frac{\partial f}{\partial \theta} \bigg) + \frac{1}{\sin^2 \theta} \frac{\partial^2 f}{\partial \phi^2}
\end{equation}
By using same condition on the circle, let us consider homogeneous harmonic functions $f(r,\theta,\phi) = r^l g(\theta,\phi) $ on $\mathbb{R}^2$. The solution of Laplace equation in spherical coordinate is given by
\begin{equation}
    \Delta f = r^{l-2} \big(l(l+1)g + \Delta_{\mathrm{S}^2} g \big)
\end{equation}
Hence, the solution can be written as
\begin{equation}
    \Delta f = 0 \,\,\, \text{iff} \,\,\, \Delta_{\mathrm{S}^2} g = -l(l+1) g
\end{equation}
where $g$ is an eigenfunction of $\Delta_{\mathrm{S}^2}$ for eigenvalue $-l(l+1)$. By using separation of variables method, we can get $g(\theta,\phi) = P(\theta)T(\phi)$, the Laplacian is written as the following
\begin{equation}
    \frac{T}{\sin \theta}\frac{\partial}{\partial \theta} \bigg(\sin \theta \frac{\partial P}{\partial \theta}\bigg) + \frac{P}{\sin^2 \theta} \frac{\partial^2 T}{\partial \phi^2} = -l(l+1) P T
\end{equation}
Dividing by $PT$ and multiplying by $\sin^2 \theta$, we will have
\begin{equation}
    \frac{\sin \theta}{P}\frac{\partial}{\theta} \bigg(\sin \theta \frac{\partial P}{\partial \theta}\bigg) + l(l+1) \sin^2 \theta = -\frac{1}{T} \frac{\partial^2 T}{\partial \phi^2} 
\end{equation}
Both function $P$ and $T$ are independent function, by finding solution of this equality with some constants $k^2$, the solution for $T$ is given by two functions $T(\phi) = \sin k \phi$ and $T(\phi) = \cos k \phi$. For the other equation, we have to solve the equation
\begin{equation}
     \sin \theta \frac{\partial}{\partial\theta} \bigg(\sin \theta \frac{\partial P}{\partial \theta}\bigg) + l(l+1) \sin^2 \theta P -k^2 P = 0
\end{equation}
This equation is is the variant of Legendre's equation. If we write $x = \cos \theta$ and consider $P(\theta) = u(\cos \theta)$, we arrive to the general Legendre equation
\begin{equation} \label{general Legendre}
    (1-x^2)u'' - 2xu' + \bigg(l(l+1) - \frac{k^2}{1-x^2} \bigg)u = 0
\end{equation}
By using subtitution $u(x) = (1-x^2)^{\frac{k}{2}}v(x)$, we get
\begin{equation}\label{general Legendre 2}
    (1 - x^2)v'' - 2(k+1)xv' + \big(l(l+1) - k(k+1)\big)v= 0
\end{equation}
when $k=0$ we get Legendre equation
\begin{equation}
(1-x)^2v'' - 2xv' + l(l+1)v = 0   
\end{equation}
which the general solution is very well known as Legendre polynomials and can be written  by using Rodrigues formula
\begin{equation}
v(x) = P_l (x) = \frac{1}{2^l l!}\frac{d^l}{dx^l} (x^2-1)^l
\end{equation}
These solution exist for $l\in \mathbb{N}_0$. If we look the equation \ref{general Legendre 2} carefully, and differentiate with respect to $x$ we will have recursive relation, that means, if we have Legendre polynomials $P_l(x)$ as the solution for $k=0$ then we will have $\frac{d}{dx} P_l(x)$ for $k=1$. Therefore, the solution of equation \ref{general Legendre} can be written as the following
\begin{equation}
    u(t) = (1-x^2)^{\frac{k}{2}} \frac{d^k}{dx^k}P_l(x)
\end{equation}
where this function is called an associated Legendre polynomials for degree $l$ and order $k$ and it is easy to show $P_l^k(x) = 0$ if $k > l$. Legendre and associated Legendre polynomials play an important role in the structure of sensing matrices constructed from spherical harmonics and Wigner D-functions.  If we consider our original problem $P(\theta) = u(\cos \theta) = P^{k}_l(\cos \theta)$ and $T(\phi) = \sin k \phi$ or $\cos k \phi$; then the complete solution of Laplace equation is given by the set of functions
\begin{equation}
    f(r,\theta,\phi) = r^l \cos k \phi P^{k}_l (\cos \theta) \,\,\, \text{and} \,\,\, f(r,\theta,\phi) = r^l \sin k \phi P^{k}_l (\cos \theta)
\end{equation}
which are called the eigenfunctions of the Laplacian on the unit sphere with eigenvalue $-l(l+1)$. It is trivial to show those functions are mutually orthogonal and then imply linearly independent functions. These function in general called real spherical harmonics and can be extended into complex spherical harmonics by using Euler formula for trigonometric function. 

It is already explained that spherical harmonics is the solution of Laplace equation on the unit sphere $\mathrm{S}^2$. Now if we consider the solution of the Laplace equation on the rotation group $\mathrm{SO(3)}$ the same approach as in $\mathrm{S}^2$ can be used. Let us define $\Delta_{\mathrm{SO(3)}}$ as the Laplace equation on the rotation group and is given by
\begin{equation}
    \Delta_{\mathrm{SO(3)}} = \frac{1}{\sin^2 \theta}\bigg(\frac{\partial^2}{\partial \phi^2} - 2\cos \theta \frac{\partial^2}{\partial \phi \partial\chi} + \frac{\partial^2}{\partial \chi^2}\bigg) + \frac{\partial^2}{\partial \theta^2} + \cot \theta \frac{\partial}{\partial \theta}
\end{equation}
Let us first define $D(\theta,\phi,\chi) \in \mathrm{SO(3)}$ parameterize by using Euler angles. Hence, the goal is to find eigenfunction on the rotation group $D(\theta,\phi,\chi)$ and its eigenvalue. By using separation variables we can write $D(\theta,\phi,\chi) = d_1(\theta)d_2(\phi)d_3(\chi)$. This separation variables reduce the partial differential equation into three Sturm-Liouville problems
\begin{equation}
    d''_2 + k^2d_2 = 0 \,\,\text{and} \,\,d''_3 + n^2d_3 = 0
\end{equation}
and the condition $d_2(0) = d_2(2\pi)\,\,\,, d'_2(0) = d'_2(2\pi)$ and $d_3(-2\pi) = d_3(2\pi)\,\,\,, d'_3(-2\pi) = d'_3(2\pi)$. The solution of $d_1$ and $d_2$ is trivial and we can write as $d_2=e^{-ik\phi}$ and $d_3 = e^{-in\chi}$. For the last Sturm-Liouville problem, we have
\begin{equation}
    (\sin \theta d'_1)' + \bigg( l(l+1)\sin \theta - \frac{n^2 - 2kn\cos\theta + k^2}{\sin \theta}  \bigg) d_1 = 0
\end{equation}
and $d_1(0)=d_1(\pi) \,\,\,, d'_1(0) = d'_1(\pi)$. In order to solve the equation for $ d_1$, let assume $x = \cos \theta$ and obtain the following equation 
\begin{equation}
    (1-x^2)''_1 - 2xd'_1 + \bigg( l(l+1) - \frac{(n-k)^2}{2(1-x)} - \frac{(n+k)^2}{2(1+x)} \bigg) d_1 = 0
\end{equation}
The solution of the differential equation for $d_1$ is given by Rodrigues formula
\begin{equation}
    d_1(x) = \frac{(-1)^{l-n}}{2^l}\sqrt{\frac{(l+k)!}{(l-n)!(l+n)!(l-k)!}}\sqrt{\frac{(1-x)^{n-k}}{(1+x)^{n+k}}} \frac{d^{l-k}(1-x)^{l+n}}{d x^{l-k}(1+x)^{n-l}}
\end{equation}
This solution will be called Wigner d-function $d_{l}^{k,n}(x) = d_1(x)$. This function can also be written in term of Jacobi polynomials.
\begin{equation}
\mathrm{d}_l^{k,n}(\cos \theta)= \omega \sqrt{\gamma} \sin^{\xi} \bigg(\frac{\theta}{2}\bigg)\cos^{\lambda}\bigg(\frac{\theta}{2}\bigg) P_{\alpha}^{(\xi,\lambda)}(\cos \theta)
\end{equation}
where $\gamma=\frac{\alpha!(\alpha + \xi + \lambda)!}{(\alpha+\xi)!(\alpha+\lambda)!}$, $\xi=\abs{k-n}$, $\lambda=\abs{k+n}$, $\alpha=l-\big(\frac{\xi+\lambda}{2}\big)$ and 
\begin{equation*}
 \omega= \begin{cases*} 
        1  & if $n\geq k $ \\
        (-1)^{n-k} & if $n<k$ 
                \end{cases*}
\end{equation*}
with degree $0 \leq l \leq \infty $ and order $-l \leq k,n \leq l$, $\forall l\in \mathbb{N}, k,n\in \mathbb{Z} $. The function $P_{\alpha}^{(\xi,\lambda)}$ is the Jacobi polynomial. 
Quantum wave equations...
\subsection{Associated Legendre Polynomials and Legendre Polynomials}
Legendre polynomials satisfy orthogonality relation on $L^2$ as the following
\begin{equation}
\int_{-1}^{1} P_l(x) P_{\hat{l}}(x) dx= \frac{2}{2l+1}\delta_{l\hat{l}}
\end{equation}
It is obvious from the last equation, the $L^2$ norm of Legendre polynomials can be calculated. In addition, the associated Legendre polynomials also satisfy orthogonal relation 
\begin{equation}
\int_{-1}^{1} P^{k}_l(x) P^{\hat{k}}_{\hat{l}}(x)dx = \frac{2}{2l+1}\frac{(l+k)!}{(l-k)!}\delta_{l\hat{l}}
\end{equation}
Legendre and associated Legendre polynomials have symmetry property as the following 
\[
 P_{l}^k(-x)=(-1)^{k+l}P_l^k(x)
\]
\[
 P_{l}^{-k}(x)=(-1)^{k}\frac{(l-k)!}{(l+k)!}P_l^k(x)
\]
In this article, the summation of Legendre polynomials is written by the expansion of Legendre polynomials which are explicitly given as:
\begin{equation}
 P_n(x) = 2^n \sum_{k=0}^{n} \binom{n}{k} \binom{\frac{n+k-1}{2}}{n}x^k
\label{eq:Legendre_exp}
 \end{equation}
For the input $x=1$, Legendre polynomials can be given as $P_{l}(1) = 0$ and $x=-1$ could be generated by the symmetry relation of Legendre polynomials. Moreover, for even $n$:
 \[
  P_n(0) = \frac{(-1)^{n/2}}{2^n} \binom{n}{n/2}.
 \]
The derivation of Legendre polynomials can be written also with Gauss Hypergeometric function ${}_2F_1(a,b,c,d)$.
\begin{equation}
\frac{\partial^k P_{l}(x)}{\partial x^k} = \frac{\Gamma(1 +k + l)}{2^k k! \Gamma(1 - k + l)} {}_2F_1\bigg(k - l, 1 + k + l, 1 + k, \frac{(1 - x)}{2}\bigg)
\end{equation}
For $x=1$, the relation can be written as
\begin{equation}
\frac{\partial^k P_{l}(1)}{\partial x^k} = \frac{\Gamma(1 +k + l)}{2^k k! \Gamma(1 - k + l)}  
\end{equation}
\subsection{Properties of Wigner-3j Symbols}\label{Property_Wigner3j}
Most of the results in this paper rely heavily on the properties of Wigner-3j symbols. As already discussed in \ref{sec2}, there is a relation between Clebsch-Gordan coefficients and Wigner-3j symbols and it can be seen as the linear coefficients of the product between different degree and order spherical harmonics as well as the product of different degree and order Wigner D-functions. Most of the properties describe in this paper is given in \cite{schulten1975exact,messiah1966quantum, edmonds_angular_2016}. Wigner-3j symbol is defined as the following
\begin{align}
\begin{pmatrix}
   l_1 & l_2 & l_3 \\
   k_1 & k_2 & k_3
  \end{pmatrix}
 \end{align}
Wigner-3j symbols have symmetry properties and follow even and odd permutation which keep the numerical values unchanged
\begin{align}
\begin{pmatrix}
   l_1 & l_2 & l_3 \\
   k_1 & k_2 & k_3
  \end{pmatrix} = \begin{pmatrix}
   l_2 & l_3 & l_1 \\
   k_2 & k_3 & k_1
  \end{pmatrix} = \begin{pmatrix}
   l_3 & l_1 & l_2 \\
   k_3 & k_1 & k_2
  \end{pmatrix}
  \end{align}  
while for odd permutation is given by
\begin{align}
(-1)^{l_1 + l_2 + l_3}\begin{pmatrix}
   l_1 & l_2 & l_3 \\
   k_1 & k_2 & k_3
  \end{pmatrix} = \begin{pmatrix}
   l_2 & l_1 & l_3 \\
   k_2 & k_1 & k_3
  \end{pmatrix} = \begin{pmatrix}
   l_1 & l_3 & l_2 \\
   k_1 & k_3 & k_2
  \end{pmatrix} = \begin{pmatrix}
   l_3 & l_2 & l_1 \\
   k_3 & k_2 & k_1
  \end{pmatrix}
\end{align}  
It also follows
\begin{align}
\begin{pmatrix}
   l_1 & l_2 & l_3 \\
   k_1 & k_2 & k_3
  \end{pmatrix} = (-1)^{l_1 + l_2 + l_3}\begin{pmatrix}
   l_1 & l_2 & l_3 \\
   -k_1 & -k_2 & -k_3
  \end{pmatrix}
\end{align} 
Wigner-3j symbols should follow the selection rule in order to prevent non-zero value and it is already given in \ref{sec2}. Furthermore, there is orthogonality properties for Wigner-3j symbols
\begin{align}
&\sum_{l_3,k_3}
(2 l_3 + 1)\begin{pmatrix}
   l_1 & l_2 & l_3 \\
   k_1 & k_2 & k_3
  \end{pmatrix}\begin{pmatrix}
   l_1 & l_2 & l_3 \\
   k'_1 & k'_2 & k'_3
  \end{pmatrix} = \delta_{k_1 k'_1} \delta_{k_2 k'_2}
\end{align} 
This orthogonality relation play important role for the analysis in this paper. If we consider the condition where $k_1 = -k$, $k_2 = k$, $k_3 = 0$ and $l_1 < l_2$, Wigner 3j-symbols satisfy the following identities \cite{schulten1975exact,messiah1966quantum}:
\begin{align}
&\sum_{k=-l_1}^{l_1}
\begin{pmatrix}
   l_1 & l_2 & \hat{l} \\
   -k & k & 0
  \end{pmatrix}^2 = \frac{1}{2\hat{l}+1}.\\
&\sum_{\hat{l}=\abs{l_1-l_2}}^{l_1+l_2} (2\hat{l}+1)
\begin{pmatrix}
   l_1 & l_2 & \hat{l} \\
   -k & k & 0
  \end{pmatrix}^2 = 1.\\
  &\sum_{\hat{l}=\abs{l_1-l_2}}^{l_1+l_2} (2\hat{l} + 1) \begin{pmatrix}
   l_1 & l_2 & \hat{l}\\
   0 & 0 & 0 
  \end{pmatrix}  \begin{pmatrix}
   l_1 & l_2 & \hat{l}\\
   -k & k & 0 
  \end{pmatrix} = 0 \,\,\mathrm{for}\,\, 1 \leq \abs{k} \leq l_1
 \\ &\sum_{\hat{l}=\abs{l_1-l_2}}^{l_1+l_2} (2\hat{l}+1)
\begin{pmatrix}
   l_1 & l_2 & \hat{l}\\
   0 & 0 & 0
  \end{pmatrix}^2 = \sum_{\hat{l}=\abs{l_1 -l_2} \atop l_1 + l_2 + \hat{l} = \mathrm{even} }^{l_1 + l_2 } (2\hat{l}+1) \begin{pmatrix}
   l_1 & l_2 & \hat{l}\\
   0 & 0 & 0
  \end{pmatrix}^2 = 1
\end{align}
 Note that from selection rule if $l_1 + l_2 + \hat{l}$ is an odd integer, then $\begin{pmatrix}    l_1 & l_2 & \hat{l}\\
   0 & 0 & 0
\end{pmatrix}$ is zero. 

Explicit formula for Wigner-3j symbol is not trivial, however there are several condition that make the expression easier for example the condition when $k_1 = k_2 =  k_3 = 0$ which is used mostly in this paper. Wigner-3j symbol is explicitly given by   :
\begin{equation}
\begin{aligned} \label{special_wigner3j}
\begin{pmatrix}
   l_1 & l_2 & l_3 \\
   0 & 0 & 0
  \end{pmatrix}  &=  (-1)^{L} \Biggl( \frac{(2L-2l_1)!(2L-2l_2)!(2L-2l_3)!}{(2L+1)!}\Biggr)^{\frac{1}{2}}\Biggl( \frac{L!}{(L-l_1)!(L-l_2)!(L-l_3)!}\Biggr)
\end{aligned}
\end{equation}
where $2L=l_1+l_2+l_3$ is an even integer. The explicit formula for general Wigner-3j symbol can be seen in most angular momentum literature, for example \cite{schulten1975exact,messiah1966quantum, edmonds_angular_2016}.
